# Supplementary material for: Rapid Structural Pruning of Neural Networks with Set-based Task-Adaptive Meta-Pruning
Source: arXiv:2006.12139 source file (2020-06-22)
Supplement: Supplementary file 1 [file 8_appendix.tex]

\newpage
\appendix

\section{APPENDIX}
We first introduce our structural mask generation process in Section~\ref{sub:set}. Then, in the following Section~\ref{sub:exps}, we explain the detailed experiment settings and  add more results.

\subsection{Set-based Structural Mask Generation}
\label{sub:set}
Here, we provide how we sampled masks with mask generative function $g(\cdot;\bsy\pi)$ and $e(\tilde{\textbf{X}};\bsy\theta)$ introduced in Section~\ref{subsec:rapid-pruning}.
\paragraph{Set representation}

%To start with, most network architectures for set input follow encoder-decoder structure to achieve permutation-invariant property. Thus, $e(\tilde{\textbf{X}};\bsy\theta)$ in Equation~\ref{eq:mask-generation} is formulated as below :
%\begin{align}
%\begin{split}
%e(\tilde{\textbf{X}}) = f_{D}(f_{E}(\tilde{\textbf{X}}; \bsy\theta_{E}); \bsy\theta_{D})
%\label{eq:set_func}
%\end{split}
%\end{align}
%where $f_{D}(\cdot; \bsy\theta_{D})$ is arbitrary decoder function and $f_{E}(\cdot; \bsy\theta_{E})$ is arbitrary encoder function. \shorttitle~applies SetTransformer~\citet{lee2018set} module to formulate above equation.

To begin with, in order to obtain an optimal pruned structure for the target task, we need to exploit the knowledge of the given task. Conventional pruning schemes search for the desired subnetworks through full mini-batch training, which will incur excessive training cost $\mathcal{C}$ as the data size gets bigger. On the other hand, we rapidly and precisely obtain the desired pruned structures through the dataset-level encoded representation. This procedure of obtaining a set representation $R(\tilde{\textbf{X}};\bsy\theta)$ with the set encoder $R$ parameterized by $\bsy\theta_{(\cdot)}$ can be formulated as follows:
\begin{align}
\begin{split}
R(\tilde{\textbf{X}};\bsy\theta) = f_{D}(f_{E}(\tilde{\textbf{X}}; \bsy\theta_{E}); \bsy\theta_{D})~~~s.t.~~~\tilde{\textbf{X}}\in\mathbb{R}^{B\times X_d} \sim \{\textbf{x}_i\}_{i=1}^N,~R(\tilde{\textbf{X}};\bsy\theta)\in\mathbb{R}^{r\times X_d}
\label{eq:set_func}
\end{split}
\end{align}
where $\tilde{\textbf{X}}\in\mathbb{R}^{B\times X_d}$ from $\mathcal{D}$ is a sampled task set, $B\leq N$ is the sampled batch, $X_d$ is the input dimensionality, and $r$ is the batch dimension of the set representation ($r\ll B$). We then define the set function as a stacked function of the encoder and the decoder where $f_{E}(\cdot;\bsy\theta_{E})\in\mathbb{R}^{R_d}$ is an arbitrary encoder function parameterized by $\bsy\theta_{E}$ and $f_{D}(\cdot;\bsy\theta_{D})$ is a decoder function parameterized by $\bsy\theta_{D}$. The encoder encodes the sampled task set $\tilde{\textbf{X}}$ into a $\mathbb{R}^{R_d}$-dimensional vector and a decoder regenerates them to the dataset-level representation. Throughout the paper, we use $r=1$ as the dimension of the set representation . We adopt a transformer module \citet{lee2018set} for set encoding, which is a learnable pooling neural network module with an attention mechanism as follows:
\begin{align}
\begin{split}
f_E(\cdot)=\mbox{AE}(\cdot,\mbox{AE}(\bsy\theta_E,\cdot)),~~~f_D(\cdot)=\mbox{rF}(\mbox{AE}(\mbox{Pool}_k(\bsy\theta_D))).
\label{eq:transformer}
\end{split}
\end{align}
where rF is any row-wise feedforward layer, AE is an attention-based encoder block~\citet{vaswani2017attention}, and $\mbox{Pool}_j$ is a Pooling by Multihead Attention with $k$ seed vectors~\citet{lee2018set}. AE is permutation equivariant blocks that are constructed upon Multihead Attention Block(MAB). Using Multi-head attention $Multihead$ introduced in Transformer~\citet{vaswani2017attention}, MAB block is defined as below:
\begin{align}
\begin{split}
    \mbox{MAB}(X,Y) =\mbox{LayerNorm}(H + \mbox{rF}(H))\\
\end{split}
\end{align} 
\begin{align}
\begin{split}
    \mbox{where}~ H= \mbox{LayerNorm} (X + \mbox{Multihead}(X,Y,Y))\\
\end{split}
\end{align}
given that $X,Y \in\mathbb{R}^{n\times X_d}$ and $LayerNorm$ is layer normalization~\citet{ba2016layer}. Then, Set Attention Block(SAB) can be defined as below:
\begin{align}
\begin{split}
    \mbox{SAB}(X) := \mbox{MAB}(X,X)
\end{split}
\end{align}
This enables to calculate representation of the set X which encodes the information of the interaction among elements in the set. Furthermore, SAB can be modified to Induced Set Attention Block(ISAB) with less complexity (SAB has complexity of $\mathcal{O}(n^2)$ and ISAB have complexity of $\mathcal{O}(nm)$) which is defined as:
\begin{align}
\begin{split}
    \mbox{ISAB}_m(X) := \mbox{MAB}(X,H) \in \mathbb{R}^{n\times d} 
\end{split}
\end{align}
\begin{align}
\begin{split}
\mbox{where}~ H = \mbox{MAB}(I,X) \in \mathbb{R}^{m\times d}
\end{split}
\end{align}
The inducing points $I$ is trainable. This scheme is similar to autoencoder where input is projected to low dimension. However, ISAB obtains good features that explains the given set. Then the encoder function in Equation~\ref{eq:transformer} can be reformulated as:
\begin{align}
\begin{split}
f_{E}(\tilde{\textbf{X}}; \bsy\theta_{E}) = \mbox{ISAB}_m(\mbox{ISAB}_m(\tilde{\textbf{X}}))
\label{eq:transformer}
\end{split}
\end{align}
We used $m=32$ in the experiment. Then, this encoded vector is aggregated through decoder function, reformulated as:
\begin{align}
\begin{split}
f_{D}(f_{E}(\tilde{\textbf{X}}; \bsy\theta_{E}); \bsy\theta_{D}) = \mbox{rF}(\mbox{SAB}(\mbox{PMA}_k(f_{E}(\tilde{\textbf{X}}; \bsy\theta_{E}))))
\end{split}
\end{align}
\begin{align}
\begin{split}
\mbox{where}~ \mbox{PMA}_k(\cdot) = \mbox{MAB}(S,\mbox{rF}(\cdot))\in \mathbb{R}^{k\times d}
\end{split}
\end{align}
We set $k=1$ in the experiments and $S$ is seed vector. In this process we can calculate $\mathcal{R}(\tilde{\textbf{X}};\bsy\theta)\in \mathbb{R}^{X_d}$ .

%Now, we calcuate $\textbf{o}_l\in\mathbb{R}^{X_l}$ as introduced in Equation~\ref{eq:mask-generation} and Figure~\ref{fig:method} where $X_l$ is dimension of the activation map. 

%In each layer, we calculate mask by $g_l(\textbf{o}_l;\bsy\pi_l)$ to prune out filters. We first reduce the dimension to $\tilde{\textbf{o}}_l \in\mathbb{R}^{K}$ where $K$ is the number of channels in layer $l$ by average pooling function. Then,  we genearte mask $\textbf{m}_l=g_l(\textbf{o}_l;\bsy\pi_l)$ as below:

%\begin{align}
%\begin{split}
% \bsy\pi_l\sim\prod^K_{k=1}\mbox{beta}(\pi_{l,k};\alpha/K,1)
%\label{eq:set-bbdrop}
%\end{split}
%\end{align}
%\begin{align}
%\begin{split}
% \textbf{m}_l|\bsy\pi_l,\textbf{o}_l\sim\prod^K_{k=1}\mbox{Ber}(m_{l,k};\psi_{l,k}(\gamma_{l,k}\tilde{o}_{l,k} +\beta_{l,k})),~~\mbox{where}~ m_{l,k}\in\{0,1\}
%\label{eq:set-bbdrop-m}
%\end{split}
%end{align}
%\begin{align}
%\begin{split}
%\psi_{l,k}(\cdot)=\pi_{l,k}\mbox{min}(1-\epsilon, \mbox{max}(\epsilon, \cdot)) 
%\label{eq:set-bbdrop-pi}
%\end{split}
%\end{align}

%This Beta-Bernoulli prior and $\beta_{l,k}$ induces sparsity in the generation of the mask and we follow the derivation of BBDropout~\citet{lee2018adaptive} to optimize the approximated posterior by Variational Inference.

\paragraph{Structural mask generation}

%\subsection{Set-dependent Structural Pruning using Sparsity-inducing Prior}
%\label{subsec:structural-pruning}
We now describe a mask generation function for \shorttitle. A pruning mask generator draws a channel-wise binary vector $\textbf{m}_l\in\mathbb{R}^{C_l}$ at layer $l$ from which we obtain the pruned model parameter $\bsy\omega_l=\textbf{m}_l\otimes \textbf{W}_l$. %we sample masks from sparsity inducing bayesian prior $\textbf{m}_l\sim{p}(\textbf{m}_l|R(\tilde{\textbf{X}}))$.
%For the meta network $ S $ , 
As inspired from Lee et al. \citet{lee2018adaptive}, we use the following sparsity-inducing beta-Bernoulli prior to generate a binary pruning mask at each layer, which follows Bernoulli distribution Bernoulli$(\textbf{m}_l;\bsy\pi_l)$, given the probability of parameterized beta distribution as follows:
\begin{align}
\begin{split}
\textbf{m}_l|\bsy\pi_l\sim\prod^{C_l}_{c=1}\mbox{Bernoulli}(\mbox{m}_{c,l};\pi_{c,l}),~~~
\mbox{where}~~\bsy\pi_l\sim\prod^{C_l}_{c=1}\mbox{beta}(\pi_{c,l};\alpha_l,1)
\label{eq:bbdrop}
\end{split}
\end{align}
With a learnable parameter $\alpha_l$ for the beta distribution, the model optimizes binary masks during training from a randomly sampled value from the beta distribution, to determine which neuron should be pruned. 

We extend this input-independent pruning method to sample binary masks based on the set representation of the target task, which is \textit{input-dependent}. This is different from data-dependent BBDrop~\citet{lee2018adaptive} in that \shorttitle~ generates mask per dataset, while the former generates mask per instance, thus hard to eliminate filters globally. Furthermore, while rather than searching for the compressed structure by training mini-batch instances at each iteration, we utilize a set representation to rapidly obtain a near-optimal subnetwork within a few gradient steps. With the obtained set representation $R(\tilde{\textbf{X}};\bsy\theta)$, we  calculate the activation $\textbf{O}_l=h_l(\textbf{O}_{l-1};\textbf{W}_l)$ for each layer $l$, where $h_l$ is the function of the layer $l$ (i.e. convolution) and $\textbf{O}_1=h_1(R(\tilde{\textbf{X}};\bsy\theta);\textbf{W}_1)$. We omit the layer notation $l$ for readability in following equations. Then, we can sample a structural pruning mask vector $\textbf{m}$ as follows:
\begin{align}
\begin{split}
\textbf{m}|\bsy\pi,\textbf{O}\sim\prod^{C}_{c=1}\mbox{Bernoulli}(\mbox{m}_c;\pi_c\psi(\gamma_c o_c+\beta_c,\epsilon)),~~~\mbox{s.t.}~~[o_1;...;o_C]=\mbox{Pool}(\textbf{O}),
\label{eq:set-bbdrop}
\end{split}
\end{align}
where $\gamma$ and $\beta$ are learnable scaling and shifting factors and we use an average pooling for  $\textbf{O}$ to obtain a representative value at each channel. The clamping function is formulated to  $\psi(\cdot,\epsilon)=\mbox{min}(1-\epsilon, \mbox{max}(\epsilon, \cdot))$ with a small $\epsilon>0$. Using a clamping function, we retain only the meaningful channels. We employ variational inference to approximate sparsity inducing posterior  $p(\textbf{W},\bsy\pi,\bsy\theta,\bsy\beta|\textbf{X})$. The KL-divergence term for our set-based task-adaptive pruning is as follows:
\vspace{0.1in}
\begin{align}
\begin{split}
D_{KL}[q(\textbf{m},\bsy\pi,\bsy\theta|\textbf{X})\|p(\textbf{m},\bsy\pi,\bsy\theta)] + D_{KL}[q(\bsy\beta)\|p(\bsy\beta)],~~~s.t.~~\bsy\beta\sim\mathcal{N}(\textbf{0},b\textbf{I}),
\label{eq:set-bbdrop-kl}
\end{split}
\end{align}
where $b$ is a fixed value for variance of the shifting factor $\bsy\beta$ to prevent $\bsy\beta$ from drifting far away. The first term is computed in a closed form solution~\citet{lee2018adaptive,nalisnick2016stick}. Also, we can easily compute second term. To this end, we can obtain approximated expectation for the prediction of given dataset $\mathcal{D}$: %$\{\textbf{x},\textbf{y}\}$:
\begin{align}
\begin{split}
p(\textbf{y}|\textbf{x},\textbf{W},\bsy\theta)\approx p(\textbf{y}|f(\textbf{x};\mathbb{E}_q[\textbf{m}]\otimes\textbf{W},\bsy\theta)),~~~s.t.~~\mathbb{E}_q[\textbf{m}]=\mathbb{E}_q[\bsy\pi]\cdot\psi(\bsy\gamma\mbox{Pool}(\textbf{O})+\bsy\beta,\epsilon)
\label{eq:set-bbdrop-approx}
\end{split}
\end{align}

\subsection{Experiments}
\label{sub:exps}

\paragraph{Experimental settings}
 We first introduce how we meta-trained \shorttitle~ and how we modified SNIP~\citet{lee2018snip} and MetaPruning~\citet{liu2019metapruning} to report the results of VGGNet and ResNet18 on two benchmark datasets (CIFAR-10 and SVHN).

For \shorttitle, meta-training updates $\bsy\phi=\{\textbf{W},~\bsy\pi,~\bsy\theta\}$ with learning rate 0.001, 0.01, and 0.001 with Adam optimizer and decreased by 0.1 at 50\% and 80\% of the total epoch. This learning rate setting is referred from BBDropout~\citet{lee2018adaptive} except for $\bsy\theta$. For  Algorithm~\ref{alg:main_alg}, we select $i=2000, B=640$ for VGGNet and $i=3000, B=500$ for ResNet18. We sampled same number of instances per class. We further set $N=10$ and the size of the minibatch as $32$.
In the pruning stage of \shorttitle, we used same learning rate as we used in meta training stage for VGGNet, and modified learning rate of $~\bsy\pi$ to 0.5 for ResNet18 to adjust pruning rate. 

For SNIP~\citet{lee2018snip}, in ResNet18 experiment, we excluded $1\times1$ convolution layer to be pruned to match the settings with ~\shorttitle. Additionally, we modified learning rate 0.01 to attain meaningful performance of SNIP, since SNIP (P) and SNIP recorded accuracy of 88.51\% and 85.26\%, respectively at matched learning rate 0.1. For VGGNet, we pruned weights of 16 convolution layers. For SNIP (P) we loaded pretrained weights on CIFAR-100 before pruning stage.

For MetaPruning~\citet{liu2019metapruning}, in ResNet18 experiment, we followed the ResNet50 Experiment settings only without Bottleneck blocks. For VGGNet, we pruned filters of 16 convolution layers which is same as ~\shorttitle. At searching phase, we searched architecture under FLOP constraints. The possible pruning ratio of the layers were set from 20\% to 60\% to satisfy the FLOP constraints, which was 40\% to 80\% in given setting. We followed the rest of the experimental settings in MetaPruning.

\paragraph{Experiments}

In this section, we add results of ResNet18 on SVHN in Table~\ref{tab:res2}, which were omitted due to the page limits. We referenced settings of Liu et al.~\citet{liu2017learning} and trained SVHN for 20 epochs. Other settings are same as above.

\begin{table*}
\tiny
\begin{center}
%\caption{Comparison of model.}
\caption{\small Experiment results of SVHN on ResNet18.  Details are same with the Table~\ref{tab:vgg}. } 
\small
\begin{tabular}{l|| c|c|c|c|c|c }

\hline 
\multicolumn{1}{l||}{Methods}&\multicolumn{1}{c|}{Accuracy (\%) }&\multicolumn{1}{c|}{P (\%)}&\multicolumn{1}{c|}{FLOPs}&\multicolumn{1}{c|}{Training Time }&\multicolumn{1}{c|}{Inference time}&\multicolumn{1}{c}{Expense} \\
\hline \hline

Full Network	&
94.57 $\pm$ 0.01 & 100 & x1.00 & 0.16 h & 3.30 sec & 0.24 \$\\
%(3913sec)18.5sec
\hline
Edge-Popup~\cite{ramanujan2019s}	&	
%Edge-Popup (2019)	&
92.61 $\pm$ 0.01 & 5.00 & x1.00& 0.20 h & 6.15 sec &0.29 \$\\ 

SNIP (P)~\cite{lee2018snip}	&	
95.38 $\pm$ 0.01 & 6.06 & x1.00& 0.35 h &6.64 sec &0.51 \$\\ 

SNIP~\cite{lee2018snip}	&	
94.88 $\pm$ 0.01 & 6.06 & x1.00& 0.35 h &6.64 sec &0.51 \$\\

%SNIP ~\cite{lee2018snip}&	89.60\% $\pm$  &2.0M(18.40\%)&	x1.0&1.80h(6483sec) &1.6sec\\ %29.3sec
%SNIP(Rand) ~\cite{lee2018snip}&	85.16\% $\pm$  &2.0M(18.40\%)&	x1.0&-  &-\\
\hdashline

%[19, 16, 59, 7, 6, 29, 15, 36, 195, 228, 201, 172, 487, 117, 84, 63]
Random Pruned&
 94.39 $\pm$ 0.23 & 72.17 &  x2.99&\textbf{0.08 h} &1.66 sec &\textbf{0.12 \$}\\%1913

MetaPruning~\cite{liu2019metapruning} &
94.49 $\pm$ 0.19 & 70.99 &  x2.83 & 2.41 h  &1.68 sec &3.51 \$\\%	7.8sec 3.2h+

%BBDropout ~\cite{lee2018adaptive} &93.66\% $\pm$ 	&  0.8M(7.49\%)	&  x3.51&37.8sec&1.2sec\\
BBDropout~\cite{lee2018adaptive} & 94.32 $\pm$ 0.02& 4.90 &x5.25& 0.31 h& 1.52 sec & 0.46 \$\\
%(7592sec

\hdashline

STAMP-Structure &\textbf{ 95.17 $\pm$ 0.01}  & \textbf{4.81} &x\textbf{5.47} &\textbf{0.11 h} &\textbf{1.51 sec}  &\textbf{0.16 \$}\\
STAMP&\textbf{ 95.41 $\pm$ 0.01} & \textbf{4.81} &x\textbf{5.47} &\textbf{0.11 h} &\textbf{1.51 sec}  &\textbf{0.16 \$}\\
%(2055 sec)

\end{tabular}
\label{tab:res2}
\vspace{-0.2in}
\end{center}

\end{table*}

\begin{figure}
\vspace{0.1in}
\begin{minipage}{.4\textwidth}
\begin{tabular}{c }
\hspace{-0.2in}
\includegraphics[height=3.3cm]{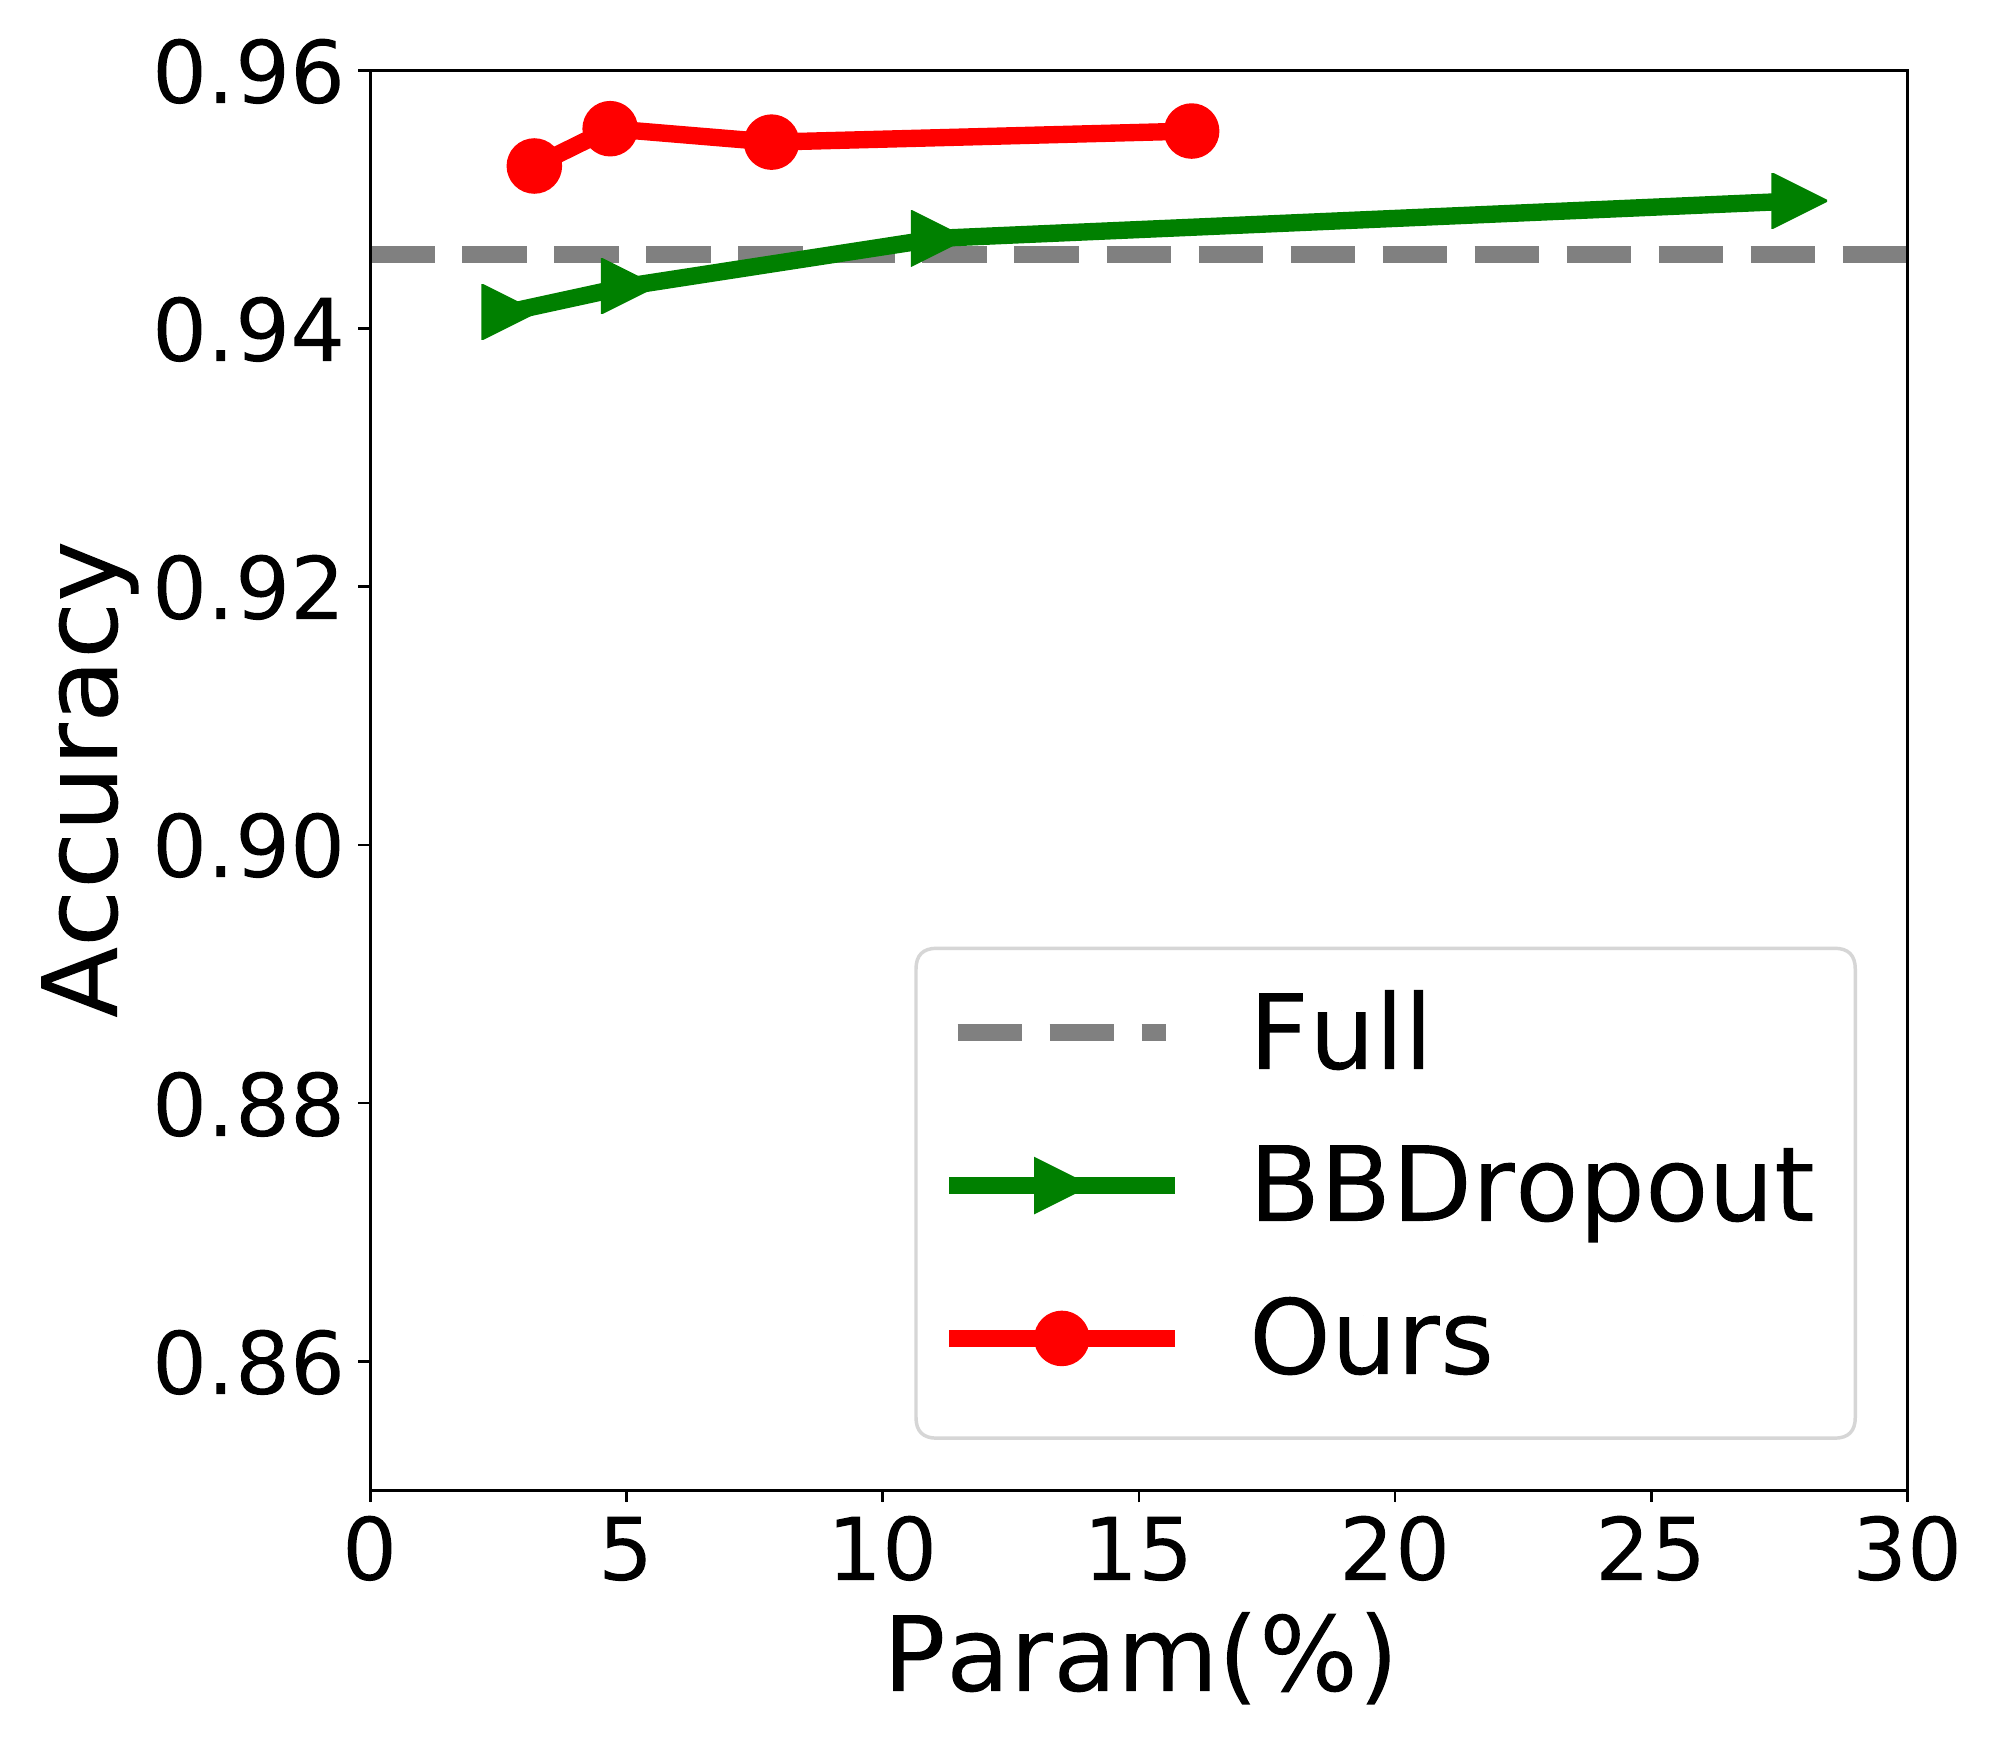}\\

%\caption{ \textbf{Accuracy over the ratio of used parameters} for SVHN on ResNet18. \textit{Full} denotes the accuracy of the ResNet18 before pruning.}

\end{tabular}
\end{minipage}
\hspace{-0.7 in}
\begin{minipage}{.65\textwidth}
\footnotesize
\begin{tabular}{l|| c|c|c|c }

\hline 
\multicolumn{1}{l||}{Methods}&\multicolumn{1}{c|}{Accuracy (\%) }&\multicolumn{1}{c|}{P (\%)}&\multicolumn{1}{c|}{FLOPs}&\parbox[c]{1.5cm}{ Training\\Time}\\
\hline \hline

Full Network	&
94.57  & 100 & x1.00 & \textbf{0.16 h} \\
%(3913sec)18.5sec
\hline

BBD ($kl$=15)& 94.70 & 11.09 &x2.86& 0.31 h\\

BBD ($kl$=20)& 94.30 & 4.86 &x5.14& 0.31 h\\
BBD ($kl$=25)& 94.12 & 2.71 &x8.62& 0.31 h\\
%(7592sec

\hdashline

STAMP ($K$=1, $kl$=15)&\textbf{ 95.44 } & \textbf{7.83} &x\textbf{4.26} &\textbf{0.11 h} \\
%(2055 sec)

STAMP ($K$=5)&\textbf{ 95.73 } & \textbf{3.84} &x\textbf{6.39} &\textbf{0.19 h} \\
STAMP ($K$=10)&\textbf{ 95.77 } & \textbf{1.81} &x\textbf{8.13} &\textbf{0.31 h} \\

%(2055 sec)

\end{tabular}

\end{minipage}
\vspace{0.1in}
\caption{\small{ \textbf{Left:} Accuracy over the ratio of used parameters for SVHN on ResNet18. \textit{Full} denotes the accuracy of the ResNet18 before pruning. \textbf{Right:} Exploring different $K$ of \shorttitle~ compared with BBDropout~\cite{lee2018adaptive}~(BBD). $kl$ is a scale factor for regularization term. }}
\label{fig:bb}
\vspace{-0.2in}
\end{figure}
We demonstrate that we accelerated the convergence of BBDropout~\citet{lee2018adaptive} by meta-training Set-based adaptation paradigm in Figure~\ref{fig:bb}. \shorttitle~ attains higher accuracy than BBDropout when same number of parameters are pruned out.
Additionally we can increase accuracy of \shorttitle~by increasing $K$ in pruning stage as seen in Figure~\ref{fig:bb}. We observe that SVHN dataset is overfitted to ResNet18 as the accuracy increases when the network is compressed. By increasing the $K$ in the pruning stage, we can attain accuracy that outperforms all of the results including that of Table~\ref{tab:res2}. Though, increasing $K$ makes ~\shorttitle~ slightly slower than the full network training time, but we observe that it is still faster than BBDropout.
